# Supplementary material for: ShadowKV: KV Cache in Shadows for High-Throughput Long-Context LLM Inference
Source: arXiv:2410.21465 source file (2025-04-25)
Supplement: Supplementary file 1 [file appendix.tex]

\section{Hello World}
%\subsection{Hello World}
